# Supplementary material for: JVNV: A Corpus of Japanese Emotional Speech with Verbal Content and Nonverbal Expressions
Source: arXiv:2310.06072 source file (2023-10-09)
Supplement: Supplementary file 1 [file appendix.tex]

\section{Emotion classifier}
% originally in proposed method
In this section, we describe the details of our emotion classifier used for assisting high-quality script selection. Although in most cases, the large language models (e.g., ChatGPT) can generate scripts conditioned on the given emotions, we still want to further improve the quality of the selected scripts. Specifically, we train an emotion classifier to assist in selecting scripts with strong emotions, filtering out those samples with incorrect or vague emotions.

In the field of emotion analysis, the WRIME ~\cite{kajiwara2021wrime} dataset is a well-known Japanese emotion analysis dataset. It contains 43k crowd-sourcing data. Each sentence was annotated by one writer and three readers. The annotations follow Plutchik’s ~\cite{plutchik1980general} eight-category emotion schema on a four-point intensity scale, ranging from 0 to 3. Finally, we define the emotion of each sentence by weighted averaging annotators' scores:
\begin{equation}
    s = \frac{s^{writer} + \frac{1}{n}\sum_{k=1}^{n}s^{reader_{k}}}{2},
\end{equation}
where $n$ is the number of reader annotators. 
If the emotion score is larger than 1, we regard the sentence as having at least weak emotion with respect to an emotion category. Under this experimental setting, we use a RoBERTa-based model to train an emotion classifier with Binary Cross Entropy loss. 

The WRIME dataset has two versions that are WRIME-ver1 and WRIME-ver2. WRIME-ver2 is a subset of WRIME-ver1 and asks another three annotators to annotate the emotion intensity together with the sentiment polarity. We also consider the extra annotations from WRIME-ver2 making the annotations more robust. After training, our emotion classifier can calculate the probability of a given sentence conveying a certain emotion. If the probability is high enough to exceed a given threshold, we claim that it expresses this emotion strongly. In this way, this probability can assist us to select those generated scripts with correct and strong emotions efficiently.

\section{Experimental Settings}
% originally in experiments
As for the LLM we used to generate scripts, we used {\tt gpt-3.5-turbo-0301} from OpenAI on March 2023. 
As for our emotion analysis model, we implemented it using PyTorch \cite{paszke2019pytorch} and also utilized Pytorch Lightning \footnote{https://pytorch-lightning.readthedocs.io/} to build the pipeline in our experiments. We downloaded the model weights of Japanese RoBERTa from Huggingface Transformers \cite{wolf-etal-2020-transformers} using {\tt rinna/japanese-roberta-base}. The Adam \cite{kingma2014adam} optimizer was used to optimize model parameters with a learning rate of $1\times10^{-4}$ and a batch size of $64$. L2-regularization with weight decay of $1\times10^{-5}$ was also applied. We trained our supervised model with $10$ epochs. We employed early stopping when the validation loss did not improve for half of the total number of epochs. 
When computing the fluency score of sentences, we compute the masked language model scores \cite{salazar-etal-2020-masked} instead of the standard perplexity of language models, which is slightly better for evaluating sentences' quality in our preliminary experiment. As for the pretrained Japanese BERT model, we used the {\tt cl-tohoku/bert-base-japanese-v2} from Huggingface Transformers for computing.

\section{Appendix}

Include extra information in the appendix. This section will often be part of the supplemental material. Please see the call on the NeurIPS website for links to additional guides on dataset publication.

\begin{enumerate}

\item Submission introducing new datasets must include the following in the supplementary materials:
\begin{enumerate}
  \item Dataset documentation and intended uses. Recommended documentation frameworks include datasheets for datasets, dataset nutrition labels, data statements for NLP, and accountability frameworks.
  \item URL to website/platform where the dataset/benchmark can be viewed and downloaded by the reviewers.
  \item Author statement that they bear all responsibility in case of violation of rights, etc., and confirmation of the data license.
  \item Hosting, licensing, and maintenance plan. The choice of hosting platform is yours, as long as you ensure access to the data (possibly through a curated interface) and will provide the necessary maintenance.
\end{enumerate}

\item To ensure accessibility, the supplementary materials for datasets must include the following:
\begin{enumerate}
  \item Links to access the dataset and its metadata. This can be hidden upon submission if the dataset is not yet publicly available but must be added in the camera-ready version. In select cases, e.g when the data can only be released at a later date, this can be added afterward. Simulation environments should link to (open source) code repositories.
  \item The dataset itself should ideally use an open and widely used data format. Provide a detailed explanation on how the dataset can be read. For simulation environments, use existing frameworks or explain how they can be used.
  \item Long-term preservation: It must be clear that the dataset will be available for a long time, either by uploading to a data repository or by explaining how the authors themselves will ensure this.
  \item Explicit license: Authors must choose a license, ideally a CC license for datasets, or an open source license for code (e.g. RL environments).
  \item Add structured metadata to a dataset's meta-data page using Web standards (like schema.org and DCAT): This allows it to be discovered and organized by anyone. If you use an existing data repository, this is often done automatically.
  \item Highly recommended: a persistent dereferenceable identifier (e.g. a DOI minted by a data repository or a prefix on identifiers.org) for datasets, or a code repository (e.g. GitHub, GitLab,...) for code. If this is not possible or useful, please explain why.
\end{enumerate}

\item For benchmarks, the supplementary materials must ensure that all results are easily reproducible. Where possible, use a reproducibility framework such as the ML reproducibility checklist, or otherwise guarantee that all results can be easily reproduced, i.e. all necessary datasets, code, and evaluation procedures must be accessible and documented.

\item For papers introducing best practices in creating or curating datasets and benchmarks, the above supplementary materials are not required.
\end{enumerate}
